# Supplementary material for: The HSIC Bottleneck: Deep Learning without Back-Propagation
Source: arXiv:1908.01580 source file (2019-12-05)
Supplement: Supplementary file 1 [file sec_supplemental2.tex]

% \subsection{Sufficient statistics} \label{ss:ssp_ssi}
This section provides all experiments figures mentioned in Section \ref{s:spp}.

\begin{figure}[ht]
  \centering
  \begin{subfigure}[b]{0.3\textwidth} \label{fig_1}
    \includegraphics[width=\textwidth]{img/EPOCH_comparison_acc.pdf}
    \caption{accuracy}
  \end{subfigure}
  \hspace{1mm}
  \begin{subfigure}[b]{0.3\textwidth} \label{fig_2}
    \includegraphics[width=\textwidth]{img/EPOCH_comparison_loss.pdf}
    \caption{loss}
  \end{subfigure}
  %JP:[is the Epoch Index label correct?] \KM:Yes I think so because there's only one training epoch during each experiment. So starting from 0 to epoch 1, but I'm not sure this is the correct way to do.  
  \caption{The performances of post-training with different pre-trained network learned by different epochs. The three experiment are trained with 5, 25, 100 epochs, labeled with ep-005, ep-025, and ep-100. This suggests that \JP{pre-training to convergence provides better post-training performance.}}
  \label{img:ssi}
\end{figure}

% \subsection{The effect of network capacity} \label{ss:ssp_cap}
\begin{figure}[ht]
  \centering
  \begin{subfigure}[b]{0.3\textwidth}
    \includegraphics[width=\textwidth]{img/FIXHID2_comparison_acc.pdf}
    \caption{Accuracy over training.}
  \end{subfigure}
  \begin{subfigure}[b]{0.3\textwidth}
    \includegraphics[width=\textwidth]{img/FIXHID2_comparison_sp_acc.pdf}
    \caption{Final accuracy of each task.}
  \end{subfigure}
  \caption{The performance of post-training with the different size of \PRETRAINED\ networks. The experiments labeled with dim-8, dim-16, dim-32, dim-64, and dim-128, is trained with the \PRETRAINED\ network of the dimension of 128 and output dimension of 8, 16, 32, 64, and 128 respectively. This reveals the large capacity network would provide more relevant information to the post-training}
  % jp comment - be careful with this, since the IB principle should be saying that only few dimensions are needed, or limited information somehow.
  \label{img:expcap}
\end{figure}

% \subsection{Multiple HSIC pre-trained networks} \label{ss:ssp_multi}
\begin{figure}[ht]
  \centering
  \begin{subfigure}[b]{0.3\textwidth}
    \includegraphics[width=\textwidth]{img/COMB_comparison_acc.pdf}
    \caption{accuracy}
    \label{img:expcomb:1}
  \end{subfigure}
  \hspace{1mm}
  \begin{subfigure}[b]{0.3\textwidth}
    \includegraphics[width=\textwidth]{img/COMB_comparison_sp_acc.pdf}
    \caption{final accuracy across tasks}
    \label{img:expcomb:2}
  \end{subfigure}
  \caption{The performance of post-training with aggregation pre-trained networks. Each task labeled with sigma-5, sigma-10, sigma-15 is post-trained with the pre-training network of sigma 5, 10, and 15 respectively. The "combine" is using all the former mentioned pre-trained, aggregated with summation to the output layer.}
  \label{img:expcomb}
\end{figure}

% \subsection{Experiments on ResNet} \label{ss:ssp_resnet}
\begin{figure}[ht]
  \centering
  \begin{subfigure}[b]{0.32\textwidth} 
    \includegraphics[width=\textwidth]{img/MOREMNIST10_comparison_acc.pdf}
    \caption{MNIST dataset}
    \label{img:expres:1}
  \end{subfigure}
  \begin{subfigure}[b]{0.32\textwidth} 
    \includegraphics[width=\textwidth]{img/MOREFMNIST10_comparison_acc.pdf}
    \caption{Fashion MNIST dataset}
    \label{img:expres:2}
  \end{subfigure}
  \begin{subfigure}[b]{0.32\textwidth} 
    \includegraphics[width=\textwidth]{img/MORECIFAR10_comparison_acc.pdf}
    \caption{CIFAR10 dataset}
    \label{img:expres:3}
  \end{subfigure}
  \caption{ResNet experiment on several datasets. In this experiment, we evaluate our work and conventional backpropagation on ResNet of 5 residual blocks. Both shows our result (labeled with ResNet-Post) is outperform the standard backpropagation training (labeled with ResNet-Backprop) at a few beginning of batch updates and final first epoch.
  \JP{The CIFAR10 result is well below state-of-the-art performance, because we are not using a convolutional architecture. Nevertheless, HSIC pretraining provides a significant boost in performance.}
  }
  \label{img:expres}
\end{figure}
